# Supplementary material for: Nonlocal Drag of Magnons in a Ferromagnetic Bilayer
Source: arXiv:1605.04336 source file (2016-05-13)
Supplement: Supplementary file 1 [file MagnonDragSuppl.pdf]

# Supplemental Material for “Nonlocal Drag of Magnons in a Ferromagnetic Bilayer”

Tianyu Liu,[1] G. Vignale,[2] and M.E. Flatté[1]

[1] *Optical Science and Technology Center and Department of Physics and Astronomy, University of Iowa, Iowa City, Iowa 52242, USA*

[2] *Department of Physics and Astronomy, University of Missouri, Columbia, Missouri 65211, USA*

## I. INTERLAYER MAGNETIC DIPOLAR INTERACTION

We consider in-plane magnetized ferromagnetic films. The position dependence of the spin-wave amplitude along the thickness direction cannot be described by plane waves. Instead, we introduce a series of orthogonal functions that satisfy the equation of motion for the magnetization, as well as the electrodynamic and exchange boundary conditions. Suppose the saturation magnetization $\mathbf{M}_S$ is along the $z$-axis and its fluctuation $\mathbf{m}$ is in the $x$-$y$ plane, as shown in Fig. 1. Making use of the Holstein-Primakoff representation of the spin operators[1] we express the magnetization in terms of bosonic operators as follows:

$$
\begin{aligned}
m^x(\mathbf{r},\xi) = \frac{1}{2}\sqrt{\frac{2\hbar\gamma M_s}{V}}\Bigg[\sum_{n\mathbf{k}}\left(a_{n\mathbf{k}} + a^\dagger_{n,-\mathbf{k}}\right)\Phi_n(\xi)e^{i\mathbf{k}\cdot\mathbf{r}} \\
-\frac{\hbar\gamma}{4M_sV}\sum_{n_1\mathbf{k}_1}\sum_{n_2\mathbf{k}_2}\sum_{n_3\mathbf{k}_3}\left(a_{n_1\mathbf{k}_1}a_{n_2\mathbf{k}_2}a^\dagger_{n_3\mathbf{k}_3} + a^\dagger_{n_1,-\mathbf{k}_1}a^\dagger_{n_2,-\mathbf{k}_2}a_{n_3,-\mathbf{k}_3}\right) \\
\times\Phi_{n_1}(\xi)\Phi_{n_2}(\xi)\Phi_{n_3}(\xi)e^{i(\mathbf{k}_1+\mathbf{k}_2-\mathbf{k}_3)\cdot\mathbf{r}}\Bigg], \\
m^y(\mathbf{r},\xi) = \frac{1}{2i}\sqrt{\frac{2\hbar\gamma M_s}{V}}\Bigg[\sum_{n\mathbf{k}}\left(a_{n\mathbf{k}} - a^\dagger_{n,-\mathbf{k}}\right)\Phi_n(\xi)e^{i\mathbf{k}\cdot\mathbf{r}} \\
-\frac{\hbar\gamma}{4M_sV}\sum_{n_1\mathbf{k}_1}\sum_{n_2\mathbf{k}_2}\sum_{n_3\mathbf{k}_3}\left(a_{n_1\mathbf{k}_1}a_{n_2\mathbf{k}_2}a^\dagger_{n_3\mathbf{k}_3} - a^\dagger_{n_1,-\mathbf{k}_1}a^\dagger_{n_2,-\mathbf{k}_2}a_{n_3,-\mathbf{k}_3}\right) \\
\times\Phi_{n_1}(\xi)\Phi_{n_2}(\xi)\Phi_{n_3}(\xi)e^{i(\mathbf{k}_1+\mathbf{k}_2-\mathbf{k}_3)\cdot\mathbf{r}}\Bigg], \\
m^z(\mathbf{r},\xi) = M_s - \frac{\hbar\gamma}{2V}\sum_{m\mathbf{k}}\sum_{n\mathbf{k}'}\left(a^\dagger_{m\mathbf{k}}a_{n\mathbf{k}'} + a_{m,-\mathbf{k}}a^\dagger_{n,-\mathbf{k}'}\right)\Phi_m(\xi)\Phi_n(\xi)e^{i(\mathbf{k}'-\mathbf{k})\cdot\mathbf{r}}, \qquad (1)
\end{aligned}
$$

where $\mathbf{r}$ is the position vector within the film plane, $\xi$ is the coordinate perpendicular to the film, $\gamma = g\mu_B/\hbar$ is the gyromagnetic ratio, $M_s$ is the saturation magnetization, $\Omega$ is the volume of a unit cell, $V$ is the volume of the film, $n$ denotes the different modes of oscillation along the thickness of the film ($x$ axis), and the orthogonal functions $\Phi_n(\xi)$ are real and will be written explicitly below.

Integrating the dipolar interaction

$$
\mathscr{H}_{dip} = \frac{\mu_0}{8\pi}\int_{d-\frac{L}{2}}^{d+\frac{L}{2}}d\xi\int d\mathbf{r}\int_{-\frac{L}{2}}^{\frac{L}{2}}d\xi'\int d\mathbf{r}'\frac{[\boldsymbol{\nabla}\cdot\mathbf{m}(\mathbf{r},\xi)][\boldsymbol{\nabla}'\cdot\mathbf{m}(\mathbf{r}',\xi')]}{\sqrt{|\mathbf{r}-\mathbf{r}'|^2+(\xi-\xi')^2}} \qquad (2)
$$

by parts, we rewrite $\mathscr{H}_{dip}$ as the magnetization in one layer interacting with the dipolar field ($\mathbf{h}_d$) in the other layer,

$$
\mathscr{H}_{dip} = \frac{\mu_0}{2}\int_{d-\frac{L}{2}}^{d+\frac{L}{2}}d\xi\int d\mathbf{r}\,\mathbf{m}(\mathbf{r},\xi)\cdot\mathbf{h}_d(\mathbf{r},\xi), \qquad (3)
$$

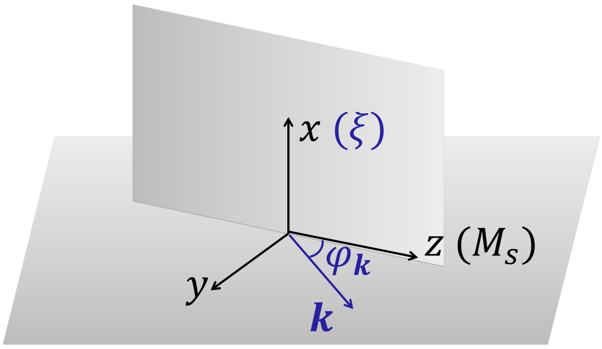


Figure 1. Reference frame in one layer: $z$ axis is always along the saturation magnetization $\mathbf{M}_s$ and $\xi$ denotes the coordinate perpendicular to the film.

where

$$\mathbf{h}_d(\mathbf{r},\xi) = \frac{\boldsymbol{\nabla}}{4\pi}\int_{\frac{L}{2}}^{\frac{L}{2}} d\xi' \int d\mathbf{r}' \frac{\boldsymbol{\nabla}'\cdot\mathbf{m}(\mathbf{r}',\xi')}{\sqrt{|\mathbf{r}-\mathbf{r}'|^2+(\xi-\xi')^2}}\,. \tag{4}$$

By performing a Fourier transform in the film plane, we obtain

$$\mathscr{H}_{dip} = -\frac{\mu_0}{2}\int_{d-\frac{L}{2}}^{d+\frac{L}{2}} d\xi \int d\mathbf{r} \int_{-\frac{L}{2}}^{\frac{L}{2}} d\xi' \int d\mathbf{r}' \sum_{\mathbf{q}} \mathbf{m}(\mathbf{r},\xi)\cdot\mathbf{G}(\xi,\xi';\mathbf{q})e^{i\mathbf{q}\cdot(\mathbf{r}-\mathbf{r}')}\cdot\mathbf{m}(\mathbf{r}',\xi')\,, \tag{5}$$

where $\mathbf{G}(\xi,\xi';\mathbf{q})$ is the tensorial Green's function. (In this, and later equations, vectors and tensors will be indicated by bold symbols, and scalars by italics.) The explicit form of $\mathbf{G}(\xi,\xi';\mathbf{q})$ is[2]

$$\mathbf{G}(\xi,\xi';\mathbf{q}) = \begin{pmatrix} G_p & iG_Q\sin\varphi_{\mathbf{q}} & -iG_Q\cos\varphi_{\mathbf{q}} \\ iG_Q\sin\varphi_{\mathbf{q}} & -G_p\sin^2\varphi_{\mathbf{q}} & \frac{1}{2}G_p\sin 2\varphi_{\mathbf{q}} \\ -iG_Q\cos\varphi_{\mathbf{q}} & \frac{1}{2}G_p\sin 2\varphi_{\mathbf{q}} & -G_p\cos^2\varphi_{\mathbf{q}} \end{pmatrix}\,, \tag{6}$$

where $G_P = (|q|/2)\exp(-|q||\xi-\xi'|)$, $G_Q = G_P\mathrm{sign}(\xi-\xi')$, and $\varphi_{\mathbf{q}}$ denotes the angle of $\mathbf{q}$ with respect to $\mathbf{M}_S$. The elements of the tensor are labeled by $G_{\alpha\beta}$ ($\alpha,\beta = x,y,z$). Substituting Eq. (1) into Eq. (5) and keeping up to quartic terms, $\mathscr{H}_{dip}$ yields both a three-magnon interaction ($\mathscr{H}^{(3)}_{dip}$) and a four-magnon interaction ($\mathscr{H}^{(4)}_{dip}$). We will use $a^\dagger$ and $b^\dagger$ to denote the creation operators in layer 1 and 2, respectively, and drop the summation over different modes, since the overlap integrals between different modes are negligible. Integrals over $\mathbf{r}$ and $\mathbf{r}'$ result in the conservation of momentum. Thus

$$\mathscr{H}^{(3)}_{dip} = -\frac{\sqrt{2M_s}}{4}\mu_0\left(\frac{\hbar\gamma}{V}\right)^{\frac{3}{2}}\sum_n\sum_{\mathbf{kq}}$$

$$\left\{a_{n,-\mathbf{q}}b^\dagger_{n,\mathbf{k}}b_{n,\mathbf{k}+\mathbf{q}}i\left[Q_{1,23}(|\mathbf{q}|)\cos\varphi_\mathbf{q}+\frac{1}{2}P_{1,23}(|\mathbf{q}|)\sin 2\varphi_\mathbf{q}\right]+c.c.\right\}$$
$$+\left\{a^\dagger_{n,\mathbf{k}}a_{n,\mathbf{k}+\mathbf{q}}b_{n,-\mathbf{q}}i\left[Q_{23,1}(|\mathbf{q}|)\cos\varphi_\mathbf{q}+\frac{1}{2}P_{23,1}(|\mathbf{q}|)\sin 2\varphi_\mathbf{q}\right]+c.c.\right\}\,, \tag{7}$$

and,

$$\begin{aligned}\mathscr{H}^{(4)}_{dip} = -\frac{\mu_0}{16}\left(\frac{\hbar\gamma}{V}\right)^2\Bigg\{&\sum_n\sum_{\mathbf{k}\mathbf{p}_1\mathbf{p}_2}\left(a_{n,\mathbf{k}}b_{n,\mathbf{p}_1}b_{n,\mathbf{p}_2}b^\dagger_{n,\mathbf{k}+\mathbf{p}_1+\mathbf{p}_2}+c.c.\right)\\
&\times\left[P_{1,234}(|\mathbf{k}|)-2Q_{1,234}(|\mathbf{k}|)\sin\varphi_\mathbf{k}+P_{1,234}(|\mathbf{k}|)\sin^2\varphi_\mathbf{k}\right]\\
&+\left(a_{n,\mathbf{k}}b^\dagger_{n,\mathbf{p}_1}b^\dagger_{n,\mathbf{p}_2}b_{n,\mathbf{p}_1+\mathbf{p}_2-\mathbf{k}}+c.c.\right)\\
&\times\left[P_{1,234}(|\mathbf{k}|)-2Q_{1,234}(|\mathbf{k}|)\sin\varphi_\mathbf{k}-P_{1,234}(|\mathbf{k}|)\sin^2\varphi_\mathbf{k}\right]\\
&+\sum_n\sum_{\mathbf{k}_1\mathbf{k}_2\mathbf{p}}\left(a_{n,\mathbf{k}_1}a_{n,\mathbf{k}_2}a^\dagger_{n,\mathbf{k}_1+\mathbf{k}_2+\mathbf{p}}b_{n,\mathbf{p}}+c.c.\right)\\
&\times\left[P_{234,1}(|\mathbf{p}|)-2Q_{234,1}(|\mathbf{p}|)\sin\varphi_\mathbf{p}+P_{234,1}(|\mathbf{p}|)\sin^2\varphi_\mathbf{p}\right]\\
&\left(a_{n,\mathbf{k}_1}a_{n,\mathbf{k}_2}a^\dagger_{n,\mathbf{k}_1+\mathbf{k}_2-\mathbf{p}}b^\dagger_{n,\mathbf{p}}+c.c.\right)\\
&\times\left[P_{234,1}(|\mathbf{p}|)-2Q_{234,1}(|\mathbf{p}|)\sin\varphi_\mathbf{p}-P_{234,1}(|\mathbf{p}|)\sin^2\varphi_\mathbf{p}\right]\Bigg\}\\
&+\frac{\mu_0}{2}\left(\frac{\hbar\gamma}{V}\right)^2\sum_n\sum_{\mathbf{k}\mathbf{p}\mathbf{q}}a^\dagger_{n,\mathbf{k}+\mathbf{q}}a_{n,\mathbf{k}}b^\dagger_{n,\mathbf{p}-\mathbf{q}}b_{n,\mathbf{p}}P_{12,34}(|\mathbf{q}|)\cos^2\varphi_\mathbf{q}\,.\end{aligned} \tag{8}$$

where

$$Q_{1,23}(|\mathbf{q}|)=\int_{d-\frac{L}{2}}^{d+\frac{L}{2}}d\xi\int_{-\frac{L}{2}}^{\frac{L}{2}}d\xi'\Phi_n(\xi-d)G_Q(q,\xi-\xi')\Phi_n(\xi')\Phi_n(\xi')\,, \tag{9}$$

$$P_{1,23}(|\mathbf{q}|)=\int_{d-\frac{L}{2}}^{d+\frac{L}{2}}d\xi\int_{-\frac{L}{2}}^{\frac{L}{2}}d\xi'\Phi_n(\xi-d)G_P(q,\xi-\xi')\Phi_n(\xi')\Phi_n(\xi')\,, \tag{10}$$

$$Q_{23,1}(|\mathbf{q}|)=\int_{d-\frac{L}{2}}^{d+\frac{L}{2}}d\xi\int_{-\frac{L}{2}}^{\frac{L}{2}}d\xi'\Phi_n(\xi-d)\Phi_n(\xi-d)G_Q(q,\xi-\xi')\Phi_n(\xi')\,, \tag{11}$$

$$P_{23,1}(|\mathbf{q}|)=\int_{d-\frac{L}{2}}^{d+\frac{L}{2}}d\xi\int_{-\frac{L}{2}}^{\frac{L}{2}}d\xi'\Phi_n(\xi-d)\Phi_n(\xi-d)G_P(q,\xi-\xi')\Phi_n(\xi')\,, \tag{12}$$

and the angle $\varphi$ is defined in Fig. 1. Similar definitions are used for four-magnon interactions. For example, $P_{1,234}(|\mathbf{q}|)$ has four $\Phi_n$ functions in the integral: one with the argument of $\xi-d$, and the other three with the argument $\xi'$. Suppose the boundaries $\xi=\pm L/2$ are symmetric, *i.e.*, they are either both "pinned" ($\mathbf{m}=0$ at the surfaces) or both "unpinned" ($\partial_\xi\mathbf{m}=0$ at the surfaces). Then for unpinned boundary conditions we have

$$\Phi_n(\xi)=\frac{\sqrt{2}}{\sqrt{1+\delta_{o,n}}}\cos[q_n(\xi+\frac{L}{2})] \tag{13}$$

with $q_n = \frac{n\pi}{L}$ , $(n = 0, 1, 2, ...)$. For pinned boundary conditions we have

$$\Phi_n(\xi) = \sqrt{2}\sin[q_n(\xi + \frac{L}{2})] \tag{14}$$

with $q_n = \frac{n\pi}{L}$ , $(n = 1, 2, ...)$.

For very thin films, only the lowest mode $n$ is excited. We choose unpinned boundary conditions, for which the lowest band is $n = 0$, then $Q_{1,23} = Q_{23,1} = Q_{1,234} = Q_{234,1} = Q(q)$ and $P_{1,23} = P_{23,1} = P_{1,234} = P_{234,1} = P_{12,34} = P(q)$. We obtain

$$\begin{aligned}\mathscr{H}^{(3)}_{dip} &= -\frac{\sqrt{2M_s}}{4}\mu_0\left(\frac{\hbar\gamma}{V}\right)^{\frac{3}{2}}\sum_{\mathbf{kp}}\left[a_{\mathbf{k}}b^\dagger_{\mathbf{p}+\mathbf{k}}b_{\mathbf{p}}i\left(Q(k)\cos\varphi_{\mathbf{k}} + \frac{1}{2}P(k)\sin 2\varphi_{\mathbf{k}}\right)\right.\\ &\left. +a^\dagger_{\mathbf{k}+\mathbf{p}}a_{\mathbf{k}}b_{\mathbf{p}}i\left(Q(p)\cos\varphi_{\mathbf{p}} + \frac{1}{2}P(p)\sin 2\varphi_{\mathbf{p}}\right) + c.c.\right] , \end{aligned}\tag{15}$$

$$\mathscr{H}^{(4)}_{dip} = -\frac{\mu_0}{2}\left(\frac{\hbar\gamma}{V}\right)^2\sum_{\mathbf{kpq}} a^\dagger_{\mathbf{k}+\mathbf{q}}a_{\mathbf{k}}b^\dagger_{\mathbf{p}-\mathbf{q}}b_{\mathbf{p}}P(q)\cos^2\varphi_{\mathbf{q}} . \tag{16}$$

where the subscript $n = 0$ has been suppressed, and we have used $\sin 2\varphi_{\mathbf{k}} = \sin 2\varphi_{-\mathbf{k}}$. Evaluating Eq. (9) and (10) yields

$$Q(q) = P(q) = \frac{1}{2qL}e^{-q(d-L)}\left(1 - e^{-qL}\right)^2 , \tag{17}$$

with $L$ being the thickness of each layer and $d$ the distance between the layers. Strictly speaking, we would need a Bogoliubov transformation which diagonalizes the quadratic terms in the full Hamiltonian and yields the exact coupled magnon modes of the bilayer. However, the mixing of magnons in different layers is small, and in the long wavelength limit $(qL \gg 1)$ we can safely skip this step: thus the amplitudes shown above are approximately the amplitudes for three- and four- magnon processes.

## II. TRANSRESISTIVITY MATRIX

The resistivity matrix connects $(\mathbf{j}_1, \mathbf{j}_{Q1}, \mathbf{j}_2, \mathbf{j}_{Q2})^T$ to $(\boldsymbol{\nabla}\mu_1, \boldsymbol{\nabla}T_1/T_1, \boldsymbol{\nabla}\mu_2, \boldsymbol{\nabla}T_2/T_2)^T$. It is convenient to define the currents $(\mathbf{J}_i)$ in terms of the regular $(\mathbf{P}_i)$ and thermal $(\mathbf{P}_{Ti})$ drift momenta of the ensemble, which are then connected to the fields $(\mathbf{F}_i)$ with the linearized Boltzmann equation, where

$$\mathbf{F}_i \equiv \begin{pmatrix}\boldsymbol{\nabla}\mu_i \\ \frac{\boldsymbol{\nabla}T_i}{T_i}\end{pmatrix} , \quad \mathbf{J}_i \equiv \begin{pmatrix}\mathbf{j}_i \\ \mathbf{j}_{Qi}\end{pmatrix} , \tag{18}$$

with $i, j = 1, 2$ labeling the layers. The magnon current density ($\mathbf{j}_i$) and the heat current density ($\mathbf{j}_{Qi}$) are readily obtained from the out-of-equilibrium magnon distribution parameterized in terms of drift momenta ($\delta n_i(\mathbf{k}) = (\partial n_i^0/\partial \epsilon_{i\mathbf{k}})\mathbf{v_k} \cdot (\mathbf{P}_i + \beta\tilde{\epsilon}_{\mathbf{k}}\mathbf{P}_{Ti})$), that is

$$\mathbf{j}_i = \sum_{\mathbf{k}} \mathbf{v_k} \frac{\partial n_i^0}{\partial \epsilon_{\mathbf{k}i}} \mathbf{v_k} \cdot (\mathbf{P}_i + \beta_i \tilde{\epsilon}_{\mathbf{k}i} \mathbf{P}_{Ti}) \;, \tag{19}$$

$$\mathbf{j}_{Qi} = \sum_{\mathbf{k}} \tilde{\epsilon}_{\mathbf{k}i} \mathbf{v_k} \frac{\partial n_i^0}{\partial \epsilon_{\mathbf{k}i}} \mathbf{v_k} \cdot (\mathbf{P}_i + \beta_i \tilde{\epsilon}_{\mathbf{k}i} \mathbf{P}_{Ti}) \,, \tag{20}$$

with $\tilde{\epsilon}_{\mathbf{k}i} \equiv \epsilon_{\mathbf{k}i} - \mu_i$. For an isotropic 2D magnon gas (short wavelength limit), the tensors involved ($\mathbf{v}_k\mathbf{v}_k$) become diagonal, and so can be written in a compact vector notation, where $\mathbf{J}_i = \underline{A}^{(i)}(\mathbf{P}_i, \mathbf{P}_{Ti})^T = \underline{A}^{(i)}\mathbf{P}^T$. Here and after, matrices with scalar elements are indicated by capital italics with underline. The matrix elements of $\underline{A}^{(i)}$ are labeled by $A^{(i)}_{\alpha\beta}$ (with $\alpha, \beta = \mu, T$). In the limit of $\epsilon_{0i} - \mu \ll k_B T$,

$$A^{(i)}_{\mu\mu} = -\frac{2n_i D}{\hbar^2} \,, \quad A_{\mu T} = A_{T\mu} = -\frac{\pi}{6\hbar^2\beta^2} \,, \quad A_{TT} = -\frac{3\zeta[3]}{\pi\hbar^2\beta^3} \,, \tag{21}$$

where $n_i$ is the density of the 2D magnon gas in layer $i$, $D$ is the exchange stiffness, $\epsilon_{0i}$ is the energy gap of the magnon dispersion in layer $i$, and $\zeta$ is the Riemann zeta function.

We then consider the "projections" of the Boltzmann equation on the regular and thermal current channels; this is done by multiplying both sides by the regular or thermal momenta and summing over $\mathbf{k}$. These two manipulations correspond to the calculation of momentum transfer rate and rate of change of heat current, respectively. The projection of the left hand side yields $\underline{A} \cdot \mathbf{F}$. The projection of the right hand side gives $-\mathbf{B} \cdot \mathbf{P}$, which is the definition of our $\mathbf{B}$ matrix. Combining the equations $\underline{A} \cdot \mathbf{F} = -\mathbf{B} \cdot \mathbf{P}$ and $\mathbf{j} = \underline{A} \cdot \mathbf{P}$ we arrive, *without any need to explicitly write down the intermediate drift momenta quantities* $\mathbf{P}$, at the desired relation between fields and currents (the generalized resistivity matrix):

$$\begin{pmatrix} \mathbf{F}_1 \\ \mathbf{F}_2 \end{pmatrix} = - \begin{pmatrix} \underline{A}^{(1)} & 0 \\ 0 & \underline{A}^{(2)} \end{pmatrix}^{-1} \begin{pmatrix} \mathbf{B}^{11} & \mathbf{B}^{12} \\ \mathbf{B}^{21} & \mathbf{B}^{22} \end{pmatrix} \begin{pmatrix} \underline{A}^{(1)} & 0 \\ 0 & \underline{A}^{(2)} \end{pmatrix}^{-1} \begin{pmatrix} \mathbf{J}_1 \\ \mathbf{J}_2 \end{pmatrix} . \tag{22}$$

Like in $A^{(i)}$, the matrix elements of $\mathbf{B}^{ij}(i, j = 1, 2)$ are labeled by $\mathbf{B}^{ij}_{\alpha\beta}\,(\alpha, \beta = \mu, T)$. They are determined by the rates of change of momentum and thermal momentum that stem from the collision terms in the Boltzmann equation. Specifically, $\mathbf{B}^{11}$ and $\mathbf{B}^{22}$ are determined by the intralayer interactions, like magnon-magnon scatterings and magnon-phonon scatterings, which do not affect the transresistivities and are not addressed in detail here. $\mathbf{B}^{12}$ is fully

determined by the interlayer collision term, which is obtained by applying Fermi's golden rule to the interlayer dipolar interaction (Eq. (15)), and will be given explicitly later. $\mathbf{B}^{21}$ can be obtained from $\mathbf{B}^{12}$ by exchanging labels 1 and 2.

When calculating the rate of change of momentum due to the interlayer collision term we come across the summation

$$\begin{aligned}&\sum_k \int d\varphi_{\mathbf{k}} \hat{\mathbf{k}}(\hat{\mathbf{k}} \cdot \mathbf{j}_i) f(k) \cos^2 \varphi_{\mathbf{k}} (1 + \sin\varphi_{\mathbf{k}})^2 \\ &= \sum_k f(k) j_i \left[ \frac{7}{16} (\hat{\mathbf{j}}_i \cdot \hat{\mathbf{M}}_S) \hat{\mathbf{M}}_S - \frac{3}{16} (\hat{\mathbf{j}}_i \times \hat{\mathbf{M}}_S) \times \hat{\mathbf{M}}_S \right] ,\end{aligned} \tag{23}$$

where vectors with hat denote the corresponding unit vectors, $f$ denotes a function that depends on the magnitude of $\mathbf{k}$, and the angular dependence comes from the anisotropy of the interlayer interaction (Eq. (15)). A similar summation appears in the calculation of the rate of change of thermal momentum. It clearly shows that $\mathbf{B}^{12}_{\alpha\beta}$ (with $\alpha, \beta = \mu, T$) are tensors in real space. Since the directions of the induced fields are taken care of by the term within the brackets in Eq. (23), we will use $B^{12}_{\alpha\beta}$ (no boldface) to denote the quantities coming from the integration over the magnitude of $\mathbf{k}$. Therefore, according to the definition of the transresistivity matrix (Eq. (1) in the main text), we obtain

$$\underline{C}^{12} = (\underline{A}^{(1)})^{-1} \underline{B}^{12} (\underline{A}^{(2)})^{-1} , \tag{24}$$

which is a scalar matrix.

We are interested in the temperature range$(\epsilon_{0i} - \mu_i)/k_B \ll T \ll T_c$, where $T_c$ is the Curie temperature—about 550 K for YIG. Within this temperature range, we have

$$(\underline{A}^{(i)})^{-1} = \frac{6\beta_i}{\pi^3 - 216 D n_i(T) \beta_i \zeta[3]} \begin{pmatrix} 18\zeta[3] & -\pi^2\beta_i \\ -\pi^2\beta_i & 12 D n_i \pi \beta_i^3 \end{pmatrix} , \tag{25}$$

where $D$ is the exchange stiffness, $n_i(T)$ is the two-dimensional magnon density of layer $i$ at temperature $T$, and the denominator

$$\pi^3 - 216 D n_i(T) \beta_i \zeta[3] \approx \pi^3 + \frac{54}{\pi} \ln \left( \frac{\epsilon_{0i} - \mu_i}{k_B T} \right) \tag{26}$$

is negative, with finite magnitude, in the limit of $\epsilon_{0i} - \mu_i \ll k_B T$.

$B^{12}$ is fully determined by the interlayer dipolar interaction. Drag resistivities due to four-magnon interactions are only 0.1% of those due to three-magnon interactions because of an extra power of the small parameter $(g\mu_B)/(La^2M_s)$, with $a$ the lattice constant. Therefore, we will drop the four-magnon interactions in the following calculations. Define a new matrix $\tilde{B}^{12}$ that satisfies

$$\begin{pmatrix} B^{12}_{\mu\mu} & B^{12}_{\mu T} \\ B^{12}_{T\mu} & B^{12}_{TT} \end{pmatrix} = \frac{2D}{\hbar}\frac{\beta\mu_0^2}{16\hbar^2}\left(\frac{g\mu_B}{L}\right)^3 \frac{M_S}{\epsilon_{02}-\mu_2} \begin{pmatrix} \tilde{B}^{12}_{\mu\mu} & \frac{\tilde{B}^{12}_{\mu T}}{\beta} \\ \frac{\tilde{B}^{12}_{T\mu}}{\beta} & \frac{\tilde{B}^{12}_{TT}}{\beta^2} \end{pmatrix}. \tag{27}$$

Such a definition has the advantage that all the matrix elements of $\tilde{B}^{12}$ have the same units, $\mathrm{m}^{-4}$. Suppose the two layers are at the same temperature. $\tilde{B}^{12}$ is simplified to be

$$\begin{aligned}\tilde{B}^{12}_{\mu\mu} =& \frac{(\epsilon_{02}-\mu_2)^2}{2\pi D^2}\int d\bar{k}\bar{k}^3\left|\bar{W}(\bar{k},\bar{d})\right|^2 \bar{\chi}_2''\left(\bar{k},\bar{k}^2+\frac{\epsilon_{01}}{\epsilon_{02}-\mu_2},T\right) n^0_{1k}\bar{n}^0_{1k} \\ &+\frac{\epsilon_{01}^2}{2\pi D^2}\int d\bar{p}\bar{p}^3\left|\bar{W}(\bar{p},\bar{d})\right|^2 \bar{\chi}_1''\left(\bar{p},\bar{p}^2+\frac{\epsilon_{02}}{\epsilon_{01}},T\right) n^0_{2p}\bar{n}^0_{2p}\,,\end{aligned} \tag{28}$$

$$\begin{aligned}\tilde{B}^{12}_{\mu T} =& \beta\Bigg\{\frac{(\epsilon_{02}-\mu_2)^3}{4\pi D^2}\int d\bar{k}\bar{k}\left|\bar{W}(\bar{k},\bar{d})\right|^2\Bigg\{2\bar{k}^2\bar{\chi}_{2\epsilon}''\left(\bar{k},\bar{k}^2+\frac{\epsilon_{01}}{\epsilon_{02}-\mu_2},T\right) \\ &+\left[2\bar{k}^2+\left(\bar{k}^2+\frac{\epsilon_{01}}{\epsilon_{02}-\mu_2}\right)^2\right]\bar{\chi}_2''\left(\bar{k},\bar{k}^2+\frac{\epsilon_{01}}{\epsilon_{02}-\mu_2},T\right)\Bigg\} n^0_{1k}\bar{n}^0_{1k} \\ &+\frac{\epsilon_{01}^3}{2\pi D^2}\int d\bar{p}\bar{p}^3\left|\bar{W}(\bar{p},\bar{d})\right|^2\left(\bar{p}^2+\frac{\epsilon_{02}-\mu_2}{\epsilon_{01}}\right)\bar{\chi}_1''\left(\bar{p},\bar{p}^2+\frac{\epsilon_{02}}{\epsilon_{01}},T\right) n^0_{2p}\bar{n}^0_{2p}\Bigg\}\,,\end{aligned} \tag{29}$$

$$\begin{aligned}\tilde{B}^{12}_{T\mu} =& \beta\Bigg\{\frac{(\epsilon_{02}-\mu_2)^3}{2\pi D^2}\int d\bar{k}\bar{k}^3\left|\bar{W}(\bar{k},\bar{d})\right|^2\left(\bar{k}^2+\frac{\epsilon_{01}}{\epsilon_{02}-\mu_2}\right) \\ &\times\bar{\chi}_2''\left(\bar{k},\bar{k}^2+\frac{\epsilon_{01}}{\epsilon_{02}-\mu_2},T\right) n^0_{1k}\bar{n}^0_{1k} \\ &+\frac{\epsilon_{01}^3}{4\pi D^2}\int d\bar{p}\bar{p}\left|\bar{W}(\bar{p},\bar{d})\right|^2\Bigg\{2\bar{p}^2\bar{\chi}_{1\epsilon}''\left(\bar{p},\bar{p}^2+\frac{\epsilon_{02}}{\epsilon_{01}},T\right) \\ &+\left[2\bar{p}^2+\left(\bar{p}^2+\frac{\epsilon_{02}}{\epsilon_{01}}\right)^2\right]\bar{\chi}_1''\left(\bar{p},\bar{p}^2+\frac{\epsilon_{02}}{\epsilon_{01}},T\right)\Bigg\} n^0_{2p}\bar{n}^0_{2p}\Bigg\}\,,\end{aligned} \tag{30}$$

$$\begin{aligned}\tilde{B}^{12}_{TT} =& \beta^2\Bigg\{\frac{(\epsilon_{02}-\mu_2)^4}{4\pi D^2}\int d\bar{k}\bar{k}\left|\bar{W}(\bar{k},\bar{d})\right|^2\left(\bar{k}^2+\frac{\epsilon_{01}}{\epsilon_{02}-\mu_2}\right) \\ &\times\Bigg\{2\bar{k}^2\bar{\chi}_{2\epsilon}''\left(\bar{k},\bar{k}^2+\frac{\epsilon_{01}}{\epsilon_{02}-\mu_2},T\right) \\ &+\left[2\bar{k}^2+\left(\bar{k}^2+\frac{\epsilon_{01}}{\epsilon_{02}-\mu_2}\right)^2\right]\bar{\chi}_2''\left(\bar{k},\bar{k}^2+\frac{\epsilon_{01}}{\epsilon_{02}-\mu_2},T\right)\Bigg\} n^0_{1k}\bar{n}^0_{1k}\end{aligned}$$

$$+\frac{\epsilon_{01}^4}{4\pi D^2}\int d\bar{p}\bar{p}\left|\bar{W}(\bar{p},\bar{d})\right|^2\left(\bar{p}^2+\frac{\epsilon_{02}}{\epsilon_{01}}\right)\left\{2\bar{p}^2\bar{\chi}''_{1\epsilon}\left(\bar{p},\bar{p}^2+\frac{\epsilon_{02}}{\epsilon_{01}},T\right)\right.$$

$$\left.+\left[2\bar{p}^2+\left(\bar{p}^2+\frac{\epsilon_{02}}{\epsilon_{01}}\right)^2\right]\bar{\chi}''_1\left(\bar{p},\bar{p}^2+\frac{\epsilon_{02}}{\epsilon_{01}},T\right)\right\}n_{2p}^0\bar{n}_{2p}^0\Bigg\}\,, \tag{31}$$

where $n_{ik}=\{\exp[(Dk^2+\epsilon_{0i}-\mu_i)/(k_BT)]-1\}^{-1}$ is the distribution function of magnons in layer $i$, and we have used $\mu_1=0$ since layer 1 is at thermal equilibrium. The quantities with a bar are dimensionless (for example, $\bar{k}=k/\sqrt{(\epsilon_{02}-\mu_2)/D}$ and $\bar{p}=p/\sqrt{\epsilon_{01}/D}$), except for $\bar{n}_{ik}=1+n_{ik}$ . $\bar{W}(\bar{k},\bar{d})$ is the dimensionless amplitude of the three-magnon interaction.

$$\bar{W}(\bar{k},\bar{d})=\frac{1}{\bar{k}}e^{-\bar{k}(\bar{d}-\bar{L})}(1-e^{-\bar{k}\bar{L}})^2\,, \tag{32}$$

where $\bar{d}=d\sqrt{(\epsilon_{02}-\mu_2)/D}$ is the dimensionless distance between the films, and $\bar{L}=L\sqrt{(\epsilon_{02}-\mu_2)/D}$ is the dimensionless thickness of each film. $\bar{\chi}''$ and $\bar{\chi}''_\epsilon$ denote the imaginary parts of the dimensionless magnon response functions at finite temperature,

$$\begin{aligned}\bar{\chi}''(\bar{k},\bar{\omega},T)&=4\pi D\chi''(\bar{k},\bar{\omega},T)\\&=-\frac{1}{\bar{k}}\int_0^\infty\frac{x(\epsilon_0-\mu)dx}{2k_BT\sinh^2\left[(x^2+1)\frac{\epsilon_0-\mu}{2k_BT}\right]}\\&\quad\times\left[\Theta(x-|\nu_-|)\sqrt{x^2-\nu_-^2}-\Theta(x-|\nu_+|)\sqrt{x^2-\nu_+^2}\right]\,,\end{aligned} \tag{33}$$

$$\begin{aligned}\bar{\chi}''_\epsilon(\bar{k},\bar{\omega},T)&=\frac{4\pi D}{\epsilon_0-\mu}\chi''_\epsilon(\bar{k},\bar{\omega},T)\\&=-\frac{1}{\bar{k}}\int_0^\infty\frac{x(\epsilon_0-\mu)dx}{2k_BT\sinh^2\left[(x^2+1)\frac{\epsilon_0-\mu}{2k_BT}\right]}\end{aligned} \tag{34}$$

$$\begin{aligned}&\times\left[\Theta(x-|\nu_-|)\sqrt{x^2-\nu_-^2}\left(\frac{\bar{k}^2}{6}+\frac{x^2}{3}+\frac{\bar{\omega}}{6}+\frac{\bar{\omega}^2}{6\bar{q}^2}\right)\right.\\&\left.-\Theta(x-|\nu_+|)\sqrt{x^2-\nu_+^2}\left(\frac{\bar{k}^2}{6}+\frac{x^2}{3}-\frac{\bar{\omega}}{6}+\frac{\bar{\omega}^2}{6\bar{q}^2}\right)\right]\,,\end{aligned} \tag{35}$$

with $\nu_\pm=\bar{\omega}/(2\bar{k})\pm\bar{k}/2$. The $\omega$-dependence of the response functions has been integrated out in Eqs. (28) to (31) by virtue of the energy conservations in the collision integral in the Boltzmann equation.

To study the temperature dependence of $\underline{C}^{12}$, we drop the factors that do not depend on temperature and define a new matrix $\underline{\tilde{C}}^{12}$ such that

$$\underline{\tilde{C}}^{12}=\left[\frac{9\hbar\mu_0^2}{2}\left(\frac{g\mu_B}{L}\right)^3\frac{M_S}{\epsilon_{02}-\mu_2}\right]^{-1}\underline{C}^{12}\,. \tag{36}$$

Therefore,

$$\tilde{C}^{12}_{\mu\mu} = D^2\beta^3[\Xi(T)]^{-1}\left\{\pi^4\tilde{B}^{12}_{TT} - 18\zeta[3]\left(\pi^2\tilde{B}^{12}_{T\mu} + \pi^2\tilde{B}^{12}_{\mu T} - 18\zeta[3]\tilde{B}^{12}_{\mu\mu}\right)\right\}, \tag{37}$$

$$\tilde{C}^{12}_{\mu T} = D^2\pi\beta^4[\Xi(T)]^{-1}\left\{\pi^3\tilde{B}^{12}_{T\mu} -6\left[2Dn_2(T)\pi^2\beta\tilde{B}^{12}_{TT} + 3\zeta[3]\left(\pi\tilde{B}^{12}_{\mu\mu} - 12Dn_2(T)\beta\tilde{B}^{12}_{\mu T}\right)\right]\right\}, \tag{38}$$

$$\tilde{C}^{12}_{T\mu} = D^2\pi\beta^4[\Xi(T)]^{-1}\left\{\pi^3\tilde{B}^{12}_{\mu T} -6\left[2Dn_1(T)\pi^2\beta\tilde{B}^{12}_{TT} + 3\zeta[3]\left(\pi\tilde{B}^{12}_{\mu\mu} - 12Dn_1(T)\beta\tilde{B}^{12}_{T\mu}\right)\right]\right\}, \tag{39}$$

$$\tilde{C}^{12}_{TT} = D^2\pi^2\beta^5[\Xi(T)]^{-1}\left\{\pi^2\tilde{B}^{12}_{\mu\mu} +12D\beta\left[-n_1(T)\pi\tilde{B}^{12}_{T\mu} - n_2(T)\pi\tilde{B}^{12}_{\mu T} + 12Dn_1(T)n_2(T)\beta\tilde{B}^{12}_{TT}\right]\right\}, \tag{40}$$

where $\Xi(T) = (\pi^3 - 216Dn_1(T)\beta\zeta[3])(\pi^3 - 216Dn_2(T)\beta\zeta[3])$.

In the high temperature limit ($k_BT \gg \epsilon_{0i} - \mu_i$),

$$n_i(T) = \sum_{\mathbf{k}} n_{ik} = -\frac{k_BT}{4\pi D}\ln\left(1 - e^{\frac{\epsilon_{0i}-\mu_i}{k_BT}}\right) \approx -\frac{k_BT}{4\pi D}\ln\left(\frac{\epsilon_{0i}-\mu_i}{k_BT}\right). \tag{41}$$

Substituting this approximation into Eqs. (28) to (31), we find the temperature dependence of the matrix elements $\tilde{B}^{12}_{\alpha\beta}$ ($\alpha,\beta = \mu, T$),

$$\tilde{B}^{12}_{\mu\mu} \propto T^3, \quad \tilde{B}^{12}_{\mu T} \propto T^2, \quad \tilde{B}^{12}_{T\mu} \propto T^2, \quad \tilde{B}^{12}_{TT} \propto T. \tag{42}$$

We keep only the leading order terms in high temperature expansion, i.e. $\tilde{B}^{12}_{\mu\mu}$, which goes as $T^3$, and simplify the drag resistivities as

$$\tilde{C}^{12}_{\mu\mu} = D^2\beta^3\pi^2(18\zeta[3])^2\tilde{B}^{12}_{\mu\mu}[\Theta(T)]^{-1}, \tag{43}$$

$$\tilde{C}^{12}_{\mu T} = \tilde{C}^{12}_{T\mu} = -D^2\beta^4\pi^4 18\zeta[3]\tilde{B}^{12}_{\mu\mu}[\Theta(T)]^{-1}, \tag{44}$$

$$\tilde{C}^{12}_{TT} = D^2\beta^5\pi^6\tilde{B}^{12}_{\mu\mu}[\Theta(T)]^{-1}, \tag{45}$$

where $\Theta(T) = \{\pi^2 + 54\ln(\beta\epsilon_{01})\zeta[3]\}\{\pi^2 + 54\ln[\beta(\epsilon_{02} - \mu_2)]\zeta[3]\}$.


[1] T. Holstein and H. Primakoff, Phys. Rev. **58**, 1098 (1940).

[2] B. A. Kalinikos, J. Phys. C **19**, 7013 (1986).
